# Supplementary material for: Robust Fair Clustering with Group Membership Uncertainty Sets
Source: arXiv:2406.00599 source file (2024-11-20)
Supplement: Supplementary file 1 [file appendix.tex]

\appendix
\onecolumn

\section{Useful Fact}  
\begin{fact} \label{cauch_ineq}
    For any positive real numbers $a_1,a_2,\dots, a_n$ and $b_1,b_2,\dots,b_n$, the following holds
    \begin{equation}
        \min_{i  \in [n]} \frac{a_i}{b_i} \leq \frac{a_1+a_2 + \cdots + a_n}{b_1+b_2 + \cdots + b_n } \leq \max_{i  \in [n]} \frac{a_i}{b_i}
    \end{equation}
\end{fact}
\begin{proof}
Let $\tau_{\max} = \max_{i  \in [n]} \frac{a_i}{b_i}$, therefore we have 
\begin{align*}
    \frac{a_1+a_2 + \cdots + a_n}{b_1+b_2 + \cdots + b_n } \leq \frac{\tau_{\max} (b_1+b_2 + \cdots + b_n)}{b_1+b_2 + \cdots + b_n} = \tau_{\max} 
\end{align*}
The lower bound can be proved similarly. 
\end{proof}

\section{Omitted Proofs}
\label{app:prelims}

\uncertaintyset*

\begin{proof}
% [Proof of \cref{prop:uncertaintyset}]
% \SE{the proof can be much shorter and we can almost say that it follows from the definition}
Let $\hat{\chi}$ be a feasible assignment under the given noise parameters, and let $(\hat{\cP}_h )_{h \in \cH}$ represent the partition of points where $\hat{\cP}_h = \hat{\chi}^{-1}(h)$. The set of points in $\cP_h$ that are assigned a different color $g \neq h$ by $\hat{\chi}$ is given by $\bigcup_{g \neq h} \hat{\cP}_g \cap \cP_h$. Moreover, for each color $h$, at most $\mhm$ points in $\cP_h$ are incorrectly assigned a color $h$ but belong to a color $g \neq h$. Thus, for any valid group assignment $\hat{\chi}$ no more than $\mhm$ points in $\cP_h$ are reassigned to a color $g \neq h$. Therefore, we have    % For any group $h\in\cH$, the noise parameters $\mhp$ restrict the number of points that can move from the set of points $\cP_h$ to another group $g$.
    % Thus, in any valid partition $( \hat{\cP}_h )_{h \in \cH}$ due to $\hat{\chi}$, the number of points which are mistakenly labeled as group $h$ but actually belong to a group $g$ is given by $  \cup_{g\neq h}  \hat{\cP}_g \cap \cP_h$. 
    % Since the number of such points can only be at most at most $\mhm$, we have that for any valid partition $( \hat{\cP}_h )_{h \in \cH}$, the following constraints must be satisfied.
    % Therefore, the total number of points which are incorrectly labeled as color $h$ in $\chi$ are given by  $ \sum_{g \neq h}  |\hat{\chi}^{-1}(g) \cap {\chi}^{-1}(h)  |$ which is at most $\mhm$ i.e., for any $h \in \cH,$
    % \SE{this isn't the same constraint}
    \begin{align*}
      \forall h \in \cH: |\cup_{g \in \cH : g \neq h }  \hat{\cP}_g \cap \cP_h  | \leq \mhm \implies   \forall h \in \cH: \sum_{g\in \cH: g \neq h } |  \hat{\cP}_g \cap \cP_h  | \leq \mhm
    \end{align*}
     The set of points assigned a color $g \neq h$ by $\chi$ but color $h$ by $\hat{\chi}$ is given by $ \hat{\cP}_h  \setminus \cP_h$. Moreover, for each color $h$, at most $\mhp$ points are incorrectly assigned a color $g \neq h$ by $\chi$ but actually has a color $h$. For any valid assignment $\hat{\chi}$ has no more than $\mhp$ points that are reassigned a color $h$ that were originally assigned a color $g\neq h$. Thus, we have
    % Furthermore, we know that the total number of points which has color $h$ but are mistakenly assigned a color $g$ is at most $\mhp.$ The number of such mistakes in color $h$ is given by $ |\hat{\chi}^{-1}(h)| - |\chi^{-1}(h) \cap \hat{\chi}^{-1}(h)| $ and is at most $\mhp.$
    % $\sum_{g \in \cH \setminus \{h\}} |\hat{\cP}_g \cap \cP_h|$ which is at most $\mhp$ as desired in \cref{eq:pos}. 
    \begin{align*}
    \forall h \in \cH:  |\hat{\cP}_h  \setminus \cP_h| =|\hat{\cP}_h| - |\hat{\cP}_h  \cap \cP_h| \leq  \mhp.
    \end{align*}
    This concludes the proof of the lemma.
    % , we also call this as ``flow'' from group $h$ to $g$. Therefore, for any two groups $g,h \in \cH$, the ``flow'' from a group $h$ to $g$, $ |\hat{\cP}_g \cap \cP_h|$ is at most $\mgh$ as defined in \cref{eq:pairwise}. 
\end{proof}

% \section{Omitted Proofs from \cref{sec:analysis}}
\begin{restatable}{observation}{clusteri}  \label{obs:ci_lb}
    Suppose that $(S,\phi)$ is $\trf{}$ solution to a given input instance and $u_h<1$ and $l_h>0$. Then the clustering $\{C_1,C_2,\cdots,C_{k'}\}$ of points induced by $(S,\phi)$ must satisfy the following,
    \begin{itemize}
        \item For any $i\in S$, $h \in \cH$, 
        $|C_{i,h}(\chi)| > \mhout$ where $\mhout$ is the number of points that are mistakenly assigned a color $h$ by $\chi$ but actually belong to a different color $g\neq h$. \label{cih_lowerbound}
        \item For any $i\in S$, $h \in \cH$, 
        $\sum_{g\neq h, g\in \cH} |C_{i,g}(\chi)| >  \mhin$ where $\mhin$ is the number of points that are mistakenly assigned a color $g \neq h$ but actually belong to a color $h$. \label{cih_ubound}
    \end{itemize}
\end{restatable}
\begin{proof}
    We know that since the clustering is robust fair it must satisfy the constraints in \cref{eq:robust_fair} i.e., 
    \begin{align*}
        \forall  i \in S, \forall g \in \cH : \min \frac{|C_{i,g}(\hat{\chi})|}{|C_i|} \geq l_g \implies \min {|C_{i,g}(\hat{\chi})|} >0
    \end{align*}
However, we know that there can be at most $m_g^-$ points that have incorrect group memberships from each color $g$. Therefore we have
\begin{align*}
       \forall  i \in S, \forall g \in \cH :\min {|C_{i,g}(\hat{\chi})|} >0 \implies  {|C_{i,g}({\chi})|} - m_g^- >0 
\end{align*}
Thus, we show the first part of the claim. For the next part, we start by summing over all the groups $g\in \cH$ and $g\neq h$, we get 
\begin{align*}
  \forall i \in S: \sum_{g \in \cH, g\neq h} {|C_{i,g}({\chi})|}  > \sum_{g \in \cH, g\neq h} m_g^-  \geq \mhin 
\end{align*}
The last inequality from \cref{eq:plus} i.e., $\sum_{g \in \cH, g\neq h} m_g^-  \geq \mhin$. Therefore, we get the desired bound.
 \end{proof}

\polyconstraints*
\begin{proof}
% [Proof of \cref{lemma:poly_constraints}]
Let $\{C_1,C_2,\dots,C_{k'}\}$ denote a feasible clustering to a given instance of our problem. Then each cluster $ C_i$ contains $ |C_{i,h}(\chi)| $ points from each color $ h \in \cH $ based on the given assignment function $ \chi $. From the set of points $\cP \setminus \cP_h $, representing points of color $ g \neq h $, at most $ \mhin $ points can have incorrect group memberships i.e., $\chi$ mistakenly assigned these points a color $g$ but actually belong to color $h$. Therefore, for each $ i \in S $ and $ h \in \cH $, we have
\begin{align*}
    \forall \hat{\chi} \in \cU, \quad \frac{|\cih(\hat{\chi})|}{|C_i|} \leq u_h 
&\implies \max_{\hat{\chi} \in \cU } \frac{|\cih(\hat{\chi})|}{|C_i|} \leq u_h.
\end{align*}
The first inequality is due to the fact that any feasible clustering to our problem satisfies the fairness constraints for all points in the uncertainty set $\cU$ and therefore, for the worst case $\hat{\chi}$ in $\cU$. 
% \SE{how do you know that you can add $\mhp$, shouldn't you first show that $\sum_{g \neq h} |C_{i,g}(\hat{\chi})| > \mhp$ as otherwise the ratio becomes $1> u_h$?}
However, in each cluster $C_i$, we know that the maximum number of points from color $h$ that are incorrectly labeled as $h$ but actually belong to a different group $g$ given by $\min\{\mhin,\sum_{{g \in \cH , g \neq h}} |C_{i,g}(\hat{\chi})|.$ Therefore, we can say that
\begin{align*}
    \max_{\hat{\chi} \in \cU } \frac{|\cih(\hat{\chi})|}{|C_i|} \leq u_h \implies  \frac{|\cih(\hat{\chi})| + \min \{\mhin,\sum_{{g \in \cH , g \neq h}} |C_{i,g}(\hat{\chi})| }{|C_i|} \leq u_h \implies  
 \leq  \frac{|\cih(\hat{\chi})| + \mhin}{|C_i|} \leq u_h.
\end{align*}
The last inequality is from the fact in \cref{obs:ci_lb} that $\sum_{{g \in \cH , g \neq h}} |C_{i,g}(\hat{\chi})| > \mhout $. Therefore, we get the desired bound in \cref{eq:lb}. 
We can similarly prove the lower bound in \eqref{eq:lb}   of this lemma. We know that the maximum number of points mistakenly assigned a color $h$  but actually belonging to group $ g \neq h$ is $ \min\{\mhout, C_{i,h}(\chi)\}$. However from the first part of \cref{obs:ci_lb} it is clear that, for any cluster $C_i$, we have $C_{i,h}(\chi) > \mhout$, therefore, in the worst case there exists an assignment $\hat{\chi}$ for which $ |C_{i,h}(\hat{\chi})| \geq   |C_{i,h}({\chi})| - \min \{\mhout, C_{i,h}(\chi)\}$. Therefore,  
\begin{align*}
    \forall \hat{\chi} \in \cU, \quad \frac{|\cih(\hat{\chi})|}{|C_i|} \geq l_h  \implies \min_{\hat{\chi} \in \cU } \frac{|\cih(\hat{\chi})|}{|C_i|} \geq l_h \implies \frac{|\cih({\chi})| - \mhout }{|C_i|} \geq l_h. 
\end{align*}
% \SE{Similarly, how do you know that you can subtract $\mhm$? doesn't this mean that $|\cih(\hat{\chi})| > \mhm$ and this has to happen since $0 < l_h$, }
Similarly, we can also prove the other direction. That is if \eqref{eq:lb} and \eqref{eq:ub} holds, then \cref{eq:robust_fair} also holds. This is because, for any $1\leq i\leq k'$,
\begin{align*}
    \forall h \in \cH : \frac{|\cih({\chi})| + \mhin }{|C_i|} \leq u_h \implies \forall \hat{\chi}: \frac{|\cih({\hat{\chi}})|  }{|C_i|}  \leq  \frac{|\cih({\chi})| + \mhin }{|C_i|} \leq u_h.
\end{align*}
For the case of lower bound constraints as well, we can say that any feasible group membership cannot constraint have more than $\mhout$ points are incorrectly labeled as $h$ in the cluster $C_i$. Therefore, for any $1\leq i \leq k'$,
\begin{align*}
    \forall h \in \cH : \frac{|\cih({\chi})| - \mhout }{|C_i|} \geq l_h \implies  \forall \hat{\chi} \in \cU, \quad \frac{|\cih(\hat{\chi})|}{|C_i|} \geq   \frac{|\cih({\chi})| - \mhout }{|C_i|}  \geq     l_h
\end{align*}
as desired.
Therefore, the exponential size constraints in \cref{eq:robust_fair} can be replaced by polynomial constraints in \eqref{eq:ub} and \eqref{eq:lb}. 

% \SE{I'm not sure if the constraints need to be equivalent, if they are then shouldn't the other direction also be established. This can be done briefly.}
\end{proof}

% \begin{claim}
% Suppose that $\{C_1, C_2, \dots, C_{k’}\}$ is a \emph{robust fair} clustering then for any $1 \leq i \leq k’$ and $h \in \cH$, we have (i) $\sum_{g \neq h} |C_{i,g}({\chi})| > \mhin$ and (ii) $|C_{i,h}({\chi})| > \mhout.$
% \end{claim}

\ublbobs*
\begin{proof}
% [Proof of Observation~\ref{obs:ublb}]
\sd{under editing.}
Suppose we have a clustering $\{C_1,\dots,C_{k'}\}$ )( $k' \leq k$), letting $\cih(\chi)$ denote the number of points belonging to group $\cH$ in cluster $C_i$, and applying the Fact \ref{cauch_ineq}, we get the following,
\begin{equation}\label{eq:color_proportion_bounds}
    \min\limits_{i \in [k']} \frac{|\cih(\chi)|}{|C_i|} \leq  \frac{|\cPh|}{|\cP|} \leq \max\limits_{i \in [k']} \frac{|\cih(\chi)|}{|C_i|}
\end{equation}
Suppose that $u_h < \frac{\nh+ \mhin }{n}$ for some color, then by the definition of the robust optimization problem, it is possible to have $\nh+ \mhin $ many points of color $h$ in the dataset. Accordingly, we it must be that for some color assignment $\frac{|\cPh|}{|\cP|}=\frac{\nh+ \mhin }{n}$ but \eqref{eq:color_proportion_bounds} implies that there exists some value $i \in [k']$ such that $\frac{|C^h_i|}{|C_i|} \ge  \frac{|\cPh|}{|\cP|}=\frac{\nh+ \mhin}{n}$. Therefore, $|C^h_i|> u_h |C_i|$ and therefore the solution is infeasible. The same argument can be made for the lower bound as well. 

We will now show that if $\forall h\in \cH: u_h \ge \frac{\nh+ \mhin }{n}, l_h \leq \frac{\nh-\mhout}{n}$, then the problem must be feasible. To show feasibility we simply show one feasible solution. Specifically, a solution which is always feasible is a one cluster solution that includes all of the points, i.e. $\{C_1\}=\{\cP\}$. Clearly, we have for any color $h: \frac{\nh-\mhout}{n} \leq \frac{|\cPh|}{|\cP|} \leq \frac{\nh+ \mhin}{n}$. Since the $u_h \ge \frac{\nh+\mhin }{n}, l_h \leq \frac{\nh- \mhout}{n}$, then the solution is feasible. 
\end{proof}
% \section{Omitted Proofs from \cref{sec:alg_rfc}}
% \label{app:alg}
% We start this section by making a simple observation about any \trf{} solution.
% \lowerboundci*

% \sd{edit here.}
\silesskone*
\begin{proof}
% [Proof of \cref{claim:silessk}]
    % Let $C_i^*$ denote the set of points assigned to each $i^* \in S^*$.
    % For any center $i^*$ in $S^*$ there exists a center $i$ in $S$ within a distance $2R$ if $R \geq R^*.$
    % This is true since the point $i^*$ must be removed from $\cP$ in some iteration, and there exists some $j \in \cP$ that was added to $S$ in the same iteration. Since $i^* \in \text{Ball}(j,2R)$ it implies that $d(i^*,j) \leq 2R.$ 
    We first show that the number of centers $S$ returned by \cref{alg:filtercenters} is at most $k$. 
    In each iteration of \cref{alg:filtercenters}, we know that the algorithm must cover at least one center $i^* \in S^*$ where $S^*$ denotes the optimal set of centers. Therefore the total number of iterations to mark all the points in $\cP$ is at most $k$. Therefore, we have $|S|\leq |S^*| \leq k$. 
    To prove the second part of the lemma, it suffices to show that for any $R \geq R^*$, there exists an assignment $\phi': \cP \rightarrow S$ that assigns points in $\cP$ to the centers in $S.$ Here $S$ is the set of centers returned by \textsc{GetCenters}. In \cref{lemma:existence_lemma}, we show using a non-constructive proof that, for any $R \geq R^*$, there exists a feasible solution to our problem with a cost of at most $3R.$
    We can construct a feasible solution to the LP$(S,R)$ as follows: for each point $j \in \cP$, we set $x_{i,j}=1$ if $\phi'(j)=1$ and $0$ otherwise. Clearly, $x$ satisfies the constraints \cref{lp:rfa}. Further, we know that i.e., each cluster $C_i = \phi^{-1}(i)$ satisfies the constraints in \cref{eq:lb} and \cref{eq:ub} i.e., 
    \begin{align*}
        \forall i\in S,h \in \cH:  |C_i \cap \cP^h| - \mhout \geq l_h |C_i| ,\text{ and } |C_i \cap \cP^h| + \mhin \leq u_h |C_i|. 
    \end{align*}
    However, we know that $|C_i| = \sum_{j \in \cP}x_{i,j} $ and  $|C_i \cap \cP^h|  = \sum_{j \in \cP_h}x_{i,j} $. Thus, $x$ satisfies the constraints \eqref{cons:ub_trf} and \eqref{cons:lb_trf}. Therefore, we conclude that for any $R\geq R^*$, there exists a non-empty feasible solution to LP~$(S,R)$.
    To prove the second part of the lemma, it is sufficient to show that for any $R \geq R^*$, there exists an assignment $\phi’: \cP \rightarrow S$ that maps points in $\cP$ to the centers in $S$, where $S$ is the set of centers returned by \textsc{GetCenters}. In \cref{lemma:existence_lemma}, using a non-constructive argument, we show that for any $R \geq R^*$, there exists a feasible solution $(S,\phi')$ to the problem with a cost of at most $3R$. 
    
    If such a solution $(S,\phi')$ exist then we can construct a feasible solution to the LP as follows: for each point $j \in \cP$, set $x_{i,j}=1$ if $\phi’(j)=i$ and $x_{i,j}=0$ otherwise. Clearly, this $x$ satisfies the constraints in \cref{lp:rfa}. Moreover, for each cluster $C_i = \phi^{-1}(i)$, the constraints in \cref{eq:lb} and \cref{eq:ub} are satisfied, i.e.,
\begin{equation}
    \forall i \in S, h \in \cH:  |C_i \cap \cP^h| - \mhout \geq l_h |C_i|, \quad \text{and} \quad |C_i \cap \cP^h| + \mhin \leq u_h |C_i|. \label{eq:feasiblesol}
\end{equation}
Furthermore, since $|C_i| = \sum_{j \in \cP}x_{i,j}$ and $|C_i \cap \cP^h| = \sum_{j \in \cP_h}x_{i,j}$, the assignment $x$ satisfies the constraints in \eqref{cons:ub_trf} and \eqref{cons:lb_trf} i.e., by substituting $|C_i|=\sum_{j \in \cP}x_{i,j}$ and $|C_i \cap \cP_h|=\sum_{j \in \cP_h}x_{i,j}$ in the \cref{eq:feasiblesol} we have
\begin{align*}
        \forall i \in S, h \in \cH:  \sum_{j \in \cP_h}x_{i,j} - \mhout \geq l_h \sum_{j\in \cP}x_{i,j} \quad \text{and} \quad  \sum_{j \in \cP_h}x_{i,j}  + \mhin \leq u_h \sum_{j\in \cP}x_{i,j}. 
\end{align*}
 Therefore, we conclude that for any $R \geq R^*$, there exists a non-empty feasible solution to LP~$(S,R)$.
\end{proof}
%      \begin{algorithm}[H]
%   \caption{\textsc{GetMapping}}
% \label{alg:get_mapping}
%  \textbf{Input}: {$R$, and $(S^*, \phi^*)$.}\\
% % \textbf{Parameter}: $\cP, k, d, p$\\
%  \textbf{Output}: {Set of centers $S$ along with a mapping $f: S^*\rightarrow S$ }  \\
%  % f is a many to one function.
%  \begin{algorithmic}[1] %[1] enables line numbers
%  % \STATE $\textsc{Unmarked} \gets \cP,  \textsc{Marked} \gets \emptyset$
%  \STATE $S \gets \emptyset, \textsc{Unmapped} \gets S^*$
%     % \WHILE{ $\textsc{Unmarked}!= \emptyset$}
%  \WHILE{ $\cP!= \emptyset$}
%     \STATE Pick an arbitrary $j \in \cP$, $S\gets S\cup \{j\}$
%     \FOR{ $i^* \in \textsc{Unmapped} $  }
%     \IF{ $i^* \in \text{Ball}(j,R) $}   
%     \STATE $f(i^*) = j$  \label{step:ji}
%     \STATE $ \textsc{Unmapped} \gets  \textsc{Unmapped}\setminus \{i^*\}$
%     \ENDIF
%     \ENDFOR
%     % \STATE $\textsc{Marked} \gets \textsc{Marked}\cup \text{Ball}(j,2R) $
%     % \STATE $\textsc{Unmarked} \gets \cP \setminus \textsc{Marked}$
%     \STATE $\cP \gets \cP \setminus \text{Ball}(j,2R) $
%     \ENDWHILE
%     \RETURN $f$
%  \end{algorithmic}
%  \end{algorithm}

\begin{restatable}{lemma}{existencelemma} \label{lemma:existence_lemma}
For any $R\! \geq R^*$, there exists an assignment $ \phi': \cP \!\! \rightarrow \!\! S$ that is \trf{} and at a clustering cost at most $3R$ i.e., $\text{cost}(S,\phi') \leq 3R$ where $S$ is the set of centers returned by the subroutine \textsc{GetCenters}. 
\end{restatable}    
\begin{proof}
% [Proof of \cref{lemma:existence_lemma}]
Suppose that we have an optimal solution $(S^* ,\phi^*)$ with cost $R^*.$ Let each point $j$ is assigned to some center $i^*$ by optimal assignment $\phis$, i.e., $\phis(j) =i^*.$ We show the existence of an assignment $\phi' : \cP \rightarrow S$  of original set of points $\cP$ to the set of centers $S$ returned by \cref{alg:filtercenters} such that
 (i) the assignment $\phi'$ is \trf{}, and
 (ii) $\text{cost}(S,\phi') \leq 3 R^*.$ Note that the proof is non-constructive since it assumes knowledge of the optimal solution.
 % \sd{Maybe remove the warmup and go to $3R^*$ assignment directly?}
% \paragraph{Warmup.} We begin by showing that there exists a robust fair assignment with a cost of at most $4R^*$ and we show how to improve this to $3R^*.$ Recall that in each iteration of \cref{alg:filtercenters}, when a center $i$ is added to $S$, we mark all unmarked points within a distance of $2R^*$ around $i.$ Let us consider the mapping $g:  S^* \rightarrow S$ where  $g(i^*)= i $ if some point $j \in C_i^*$ is first marked in the iteration when $i$ is added to $S$. By definition of $g$, each optimal center $i^* \in S^*$ can be assigned to exactly one center $i \in S$. Therefore, we construct the assignment $\phi'$ where $\phi'(j) = g(\phi^*(j)).$
% Clearly, each point is assigned to a center $i \in S$ within a distance of at most $4R^*$ and it is also easy to show that such an assignment is \emph{robust fair}. 
% \begin{figure}[H]
%     \centering
%     \includegraphics[scale=0.5]{Figures/figure1_alg.png}
%     \caption{In this example $g(i_1^*)=g(i_2^*)=j_1$; therefore in the worst case any point is assigned to a center at a distance of at most $4R^*$. In this example $j_3$ has $d(j_3,\phi'(j_3))= 4R^*.$ \sd{replace this figure after editing.} }
%     % \SE{it is really not clear that $d(j_3,\phi'(j_3))= 4R^*.$ from the drawing.}
%     \label{fig:alg_one}
% \end{figure}

To improve the distance to $3R^*$ we construct a new assignment $\phi'$ using the mapping $f: S^* \rightarrow S$.
% invoking the \cref{alg:get_mapping} (see \cref{sec:maxflow}) to get 
For each center $i^* \in S^*$ there is a unique center $i' \in S$ at a distance of at most $R^*$. 
Therefore, we construct a mapping $f:S^*\rightarrow S$ as follows: $f(i^*) = i$ where $d(i',i^*) \leq 2R^*.$ Notice that there is a unique $i\in S$ associated with each $i^*$ since every center $i' \in S$ has an associated center $i^* \in S^*$ since the \textsc{GetCenters} marks each center $i^* \in S^*$ when its corresponding $f^{-1}(i')$ is added to $S.$ Further, we distance $d(i',i^*) \leq 2R^*$ since the subroutine \textsc{GetCenters} only marks marks the points within a distance of $2R^*$ from $i'.$ 
% \SE{can't you say that associated with each center $i' \in S$ is at least one unique center $i^* \in S^*$ which it marked in GetCenters and this optimal center would be at a distance of at most $2R$. Just take the cluster of $i^*$ and send it to $i$.}
We construct the assignment $\phi'$ where each point $j \in \cP$ is assigned to a center $i' \in S$  where $i' = f( \phi^*(j)).$ Therefore, this assignment guarantees that (i) the set of all the points in $C_i^*$ corresponding to center $i^*$ gets assigned to the same center $i'=f(i^*)$, and (ii) each center $i' \in S$ gets assigned all the points from at least one of the optimal clusters. Finally, we prove that this new assignment $\phi'$ is both robust fair and has a cost of at most $3R^*.$ We first prove that $\text{cost}(S,\phi') \leq 3R^*$. We know that following is true for any point $j \in \cP$, 
\begin{align} 
    d(j, \phi'(j)) 
    &\leq d(j, \phis(j)) + d(\phis(j), \phi'(j)) \label{eq:1} \\  
    &\leq R^* + d(\phis(j),\phi(j)) \label{eq:2} \\ 
    &\leq R^* + 2R^* \label{eq:3} 
\end{align}
Inequalities \eqref{eq:1} follows from triangle inequality. Inequality \eqref{eq:2} follows from the fact that $\phi^*$ is optimal \trf{} assignment. Finally, inequality \eqref{eq:3} is from the fact that $d(\phi^*(j), \phi'(j)) \leq 2R^*$ by the definition of the mapping $f.$
% \begin{figure}[H]
%     \centering
%     \includegraphics[scale=0.5]{Figures/figure2_alg.png}
%     \caption{For the same example in \cref{fig:alg_one}, $f(j_1)=i_1^*, f(j_3)= i_2^*$; therefore the optimal cluster corresponding to $i_2^*$ is assigned to $j_3$ instead of $j_1$. Therefore $d(j_3,\phi'(j_3))$ is reduced to $3R^*$. \sd{Replace this figure by editing.}} 
%     \label{fig:alg_two}    
% \end{figure}
It remains to show that $(S,\phi')$ is indeed \emph{robust fair.} The following claim concludes the proof of this lemma.
\end{proof}
\begin{claim}\label{claim:robustfair}
    The clustering induced by $(S,\phi')$ is \emph{robust fair.}  
\end{claim}
% The proof of \cref{claim:robustfair} can be found in \cref{app:alg}.
\begin{proof}[Proof of \cref{claim:robustfair}]
Recall that  $C_i^* = \{j : \phi^*(j) = i^*\}$ denote the set of points that are assigned to center $i^* \in S^*$. Since $(S^*,\phi^*)$ is a optimal feasible clustering, the following is true, 
    \begin{align*}
      \forall i \in S, \forall h \in \cH ,
     u_h|C_i^*|   &\geq |C_{i,h}^*| + \mhin, \text{ and }  l_h |C_i^*|  \leq |C_{i,h}^*| - \mhout.  
    \end{align*}
    Given a set of centers $S$ and an assignment $\phi'(j) =  f(\phi^*(j)) $ and hence we can say that $C_i = \{j : \phi'(j) = i\}$ for each $i \in S$. Let $N(i) = \{i^* \in S^* : f(i^*) = i \} $, then we can say that,
    \begin{align*}
          \frac{|C_{i,h}|+\mhin}{|C_i|}  &= \frac{\big(\sum_{ i^* \in N(i) } |C_{i,h}^*|   
          \big) +\mhin }{\sum_{ i^* \in N(i) } |C_i^*|} \\  &\leq \frac{\sum_{ i^* \in N(i) } \big( |C_{i,h}^*| +  \mhin \big) }{\sum_{ i^* \in N(i) } |C_i^*|} \\ &\leq \max_{ i^* \in N(i) } \frac{|C_{i,h}^*| + \mhin}{|C_i^*|}  \leq u_h
    \end{align*}
    \begin{align*}
         \frac{|C_{i,h}|-\mhout}{|C_i|}  &= \frac{\big(\sum_{ i^* \in N(i) } |C_{i,h}^*|\big) -\mhout  }{\sum_{ i^* \in N(i) } |C_i^*|}  \\ &\geq  \frac{\sum_{ i^* \in N(i) } \big( |C_{i,h}^*| -\mhout  \big) }{\sum_{ i^* \in N(i) } |C_i^*|} \\
         &\geq \min_{i^* \in N(i)} \frac{ |C_{i,h}^*|  - \mhout   }{ |C_{i}^*|} \geq l_h
    \end{align*}
The above inequalities follow from the \cref{cauch_ineq} since for any  center $i^*\in N(i)$, $\frac{ |C_{i,h}^*|  - \mhout   }{ |C_{i}^*|} \geq  l_h $ and $\frac{ |C_{i,h}^*|  + \mhin   }{ |C_{i}^*|} \leq  u_h.$
\end{proof}
\begin{restatable}{lemma}{fairnessviolation}\label{lemma:fairness_violation}
     $(\hat{S},\hat{\phi})$ returned by  \cref{alg:lbfaircluster} is a $\lambda$-violating solution where $\lambda $ is at most $\frac{2}{\outm}.$
     % where $\outm = \sum_{h\in \cH}\mhout.$
\end{restatable}
\begin{proof}
% [Proof of \cref{lemma:fairness_violation}]
    According to $\lambda$-violating solution in \cref{eq:robust_fair_viol} is only required to satisfy the following reduced constraints.
   \begin{equation*}
 \forall i\in S, h\in \cH :  \frac{|C_{i,h}({\chi})| + \mhin }{ |C_i|} \leq  u_h +\lambda \text{ and } \frac{|C_{i,h}({\chi})|- \mhout }{ |C_i|}  \geq  l_h  -\lambda 
 \end{equation*}
 Therefore, for any given clustering $\{C_i\}_{i\in S}$, we have the fairness violation $\lambda$ as follows,
\begin{align*}
    \lambda \leq \max_{h \in \cH, i\in S} \left\{ \frac{l_h|{C}_i| - |{C}_{i,h}(\chi)| + \mhout }{|{C}_i|},  \frac{ |{C}_{i,h}(\chi)| + \mhin - u_h|{C_{i}}| }{|{C_i}|}  \right\}
\end{align*}
Let $\hat{C}_i$ denote the cluster correspond to the set of points that are assigned to center $i \in S$. To show the fairness violation for each cluster $C_i$ and color $h$ as follows, 
    \begin{align*}
   \frac{l_h|\hat{C}_i| - |\hat{C}_{i,h}| + \mhout }{|\hat{C}_i|}   \leq  \frac{l_h (|C_i^{\text{LP}} |+ 1) - (|C_{i,h}^{\text{LP}}|-1) + \mhout }{|C_i^{\text{LP}}|-1} &=  \frac{l_h |C_i^*| - ( |C_{i,h}^{\text{LP}}|-\mhout) }{|C_i^{\text{LP}}|-1} + \frac{ l_h+1 }{|C_i^{\text{LP}}|-1} \\& \leq  0 +   \frac{ l_h+1 }{|C_i^{\text{LP}}|-1} 
                % &=  \frac{ l_h+1 }{|C_i^{\text{LP}}|-1} \\
                <   \frac{ l_h+1 }{\outm} 
                % &=   \frac{ (1+ l_h) }{\outm}  
        \end{align*}
    The first inequality follows from the guarantees of the rounding algorithm described in \cref{lemma:obj_rounded}. The second inequality is due to the fact that $\textrm{x}$ is \trf{} satisfying the constraints \cref{lp:rfa}-\cref{eq:endrfa}, followed by a direct application of \cref{cih_lowerbound} i.e., $|C_i^{\text{LP}}|> \sum_{h}\mhout $. 
    % Thus, the fractional clusters must satisfy $l_h |C_i^*| - ( |C_{i,h}^*|-\mhout) \leq T|C_i^*|$  and ~\eqref{ineq:cih} respectively.
    Similarly, we also compute the following,
    \begin{align*}
        \frac{ |\hat{C}_{i,h}| + \mhin - u_h|\hat{C_{i}}| }{|\hat{C_i}|} 
                &\leq  \frac{  (|C_{i,h}^{\text{LP}}|+1) + \mhin -u_h (|C_i^{\text{LP}}| - 1) }{|C_i^{\text{LP}}|-1}  \\
                % \label{ineq:1} \\
                &=   \frac{  |C_{i,h}^{\text{LP}} -u_h |C_i^{\text{LP}}| + \mhin  }{|C_i^{\text{LP}}|-1}  + \frac{1+u_h}{|C_i^{\text{LP}}|-1}
                % \label{ineq:1}  \\
                \leq \frac{ u_h  +1 }{|C_i^{\text{LP}}|-1}  
                <\frac{ u_h  +1 }{\outm }
                % & =   \frac{ u_h  +1 }{|C_i^*|-1} \\
 % & \leq T  +  \frac{ u_h  +1+T }{\outm }
    \end{align*}
    The first inequality follows from the guarantees of the rounding algorithm in \cref{lemma:obj_rounded}. The second inequality is since the solution $\textrm{x}$ is \trf{} and satisfies the constriants \cref{lp:rfa}-\cref{eq:endrfa}. The last inequality is by using \cref{cih_lowerbound} i.e., $|C_i^{\text{LP}}|> \sum_{h}\mhout $. Finally, we have the following bound on $\lambda$,
    \begin{align*}  
    \lambda \leq  {\max_{h \in \cH} \left\{ \frac{ l_h  +1 }{\outm} ,\frac{1+u_h }{\outm} \right\} }    <  \frac{2}{\outm} 
    % & \leq  T + \mathcal{O}(1/n) \\
    \end{align*}
The last inequality is due to the fact that $l_h \leq u_h<1$. 
% Since we know that $\outm $ is at least a constant fraction of $n$, we can conclude that the \textit{maximum fairness violation} is at most $  \mathcal{O}(1/n).$
\end{proof}

\finaltheorem*
\begin{proof}
% [Proof of \cref{thm:final}]
    For any given instance of \rfc{}, any non-empty solution $(\hat{S},\hat{\phi})$ returned by \textsc{RobustAlg} (\cref{alg:lbfaircluster}) has a cost of at most $3R^*$ guaranteed by the fractional assignment returned by LP$(\hat{S},\hat{\phi})$ as no point is fractionally assigned to any center at a distance more than $3R^*$. Further, from \cref{lemma:fairness_violation} we can say that $(\hat{S},\hat{\phi})$ is a $\lambda$-violating solution with $\lambda  \leq  \frac{2}{\outm}$. This concludes the proof of the theorem.
\end{proof}

\section{Maxflow Rounding}
\label{sec:maxflow}
\begin{definition}
    A \textsc{MaxFlow} network is defined by a directed graph $G = (V,E)$, with a source vertex $s \in V$ and a sink vertex $t \in V$, where each edge $(i,j) \in E$ has a non-negative capacity $c_{i,j}$. Each vertex $v \in V$ is associated with a demand $d_v$. The goal of the problem is to find a circulation of flow in the network. 
\end{definition}

 \begin{algorithm}[H]\label{alg:fair_round}
  \caption{\textsc{MaxFlowRounding}}
 \textbf{Input}: An instance $\cI$ of \rfc{}, along with the fractional solution $x^*$ to LP$(\hat{S},R^*)$ \\
 \textbf{Output}: {Rounded solution $X$}  \\
  \begin{algorithmic}[1] %[1] enables line numbers
 \STATE Construct a \textsc{MaxFlow} flow network corresponding to the input instance of \rfc{} shown in the \cref{fig:enter-label}
 \STATE $X$ is constructed based on the flows in the corresponding \textsc{MaxFlow} network as described in \cref{lemma:rounding_final}
 \RETURN  $\{ X_{i,j}, i \in S, j\in \cP \} $
  \end{algorithmic}
 \end{algorithm}     
 
 \begin{figure}[H]
    \centering
    \includegraphics[scale=0.25]{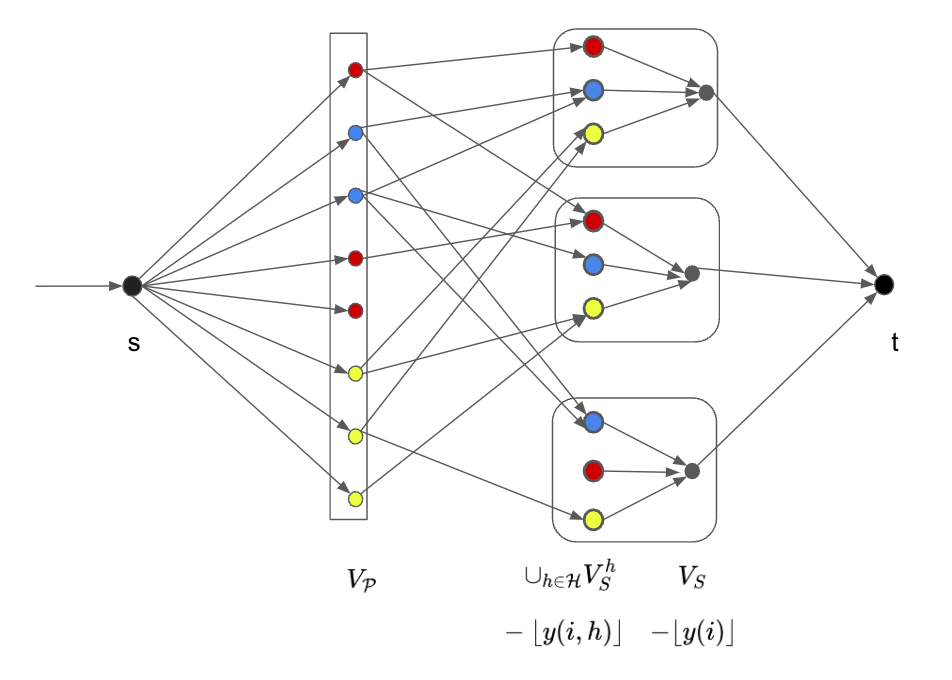}
    \caption{Example of the \textsc{MaxFlow} network corresponding to an instance of \rfa{}}
    \label{fig:enter-label}
\end{figure}

\begin{proof}
     For any point $j$, the fractional assignment vector of $j$ is given by $[x_{1,j},x_{2,j},\cdots, x_{|S|,j}]$. Let ${x}(j):= \sum_{i\in S}x_{i,j}$ denote the fractional mass of point $j$. Similarly, let $y(i):= \sum_{j \in \cP}x_{i,j}$ denote the fractional mass of points assigned to each center $i$. We define $y(i,h):= \sum_{j \in \cP^h}x_{i,j}$ analogous to $y(i)$ for each group $h \in \cH$. Finally we let $Y(i):= \lfloor y(i) \rfloor - \sum_{ h\in \cH}\lfloor y(i,h)\rfloor$ and $Y :=  n - \sum_{i \in S} \lfloor y(i) \rfloor$. 

    \paragraph{Construction of \textsc{MaxFlow} Flow network corresponding to solution $x$ and instance $\sI$.} Let us now construct \textsc{MaxFlow} flow network $F(x,\sI)$ that converts a fractional feasible solution $\{x_{i,j}:i\in S,j \in \cP\}$ satisfying constraints \cref{lp:rfa}-\cref{eq:endrfa} to a rounded solution $\{X_{i,j}\}$. This rounding method has been studied for assignment problems in \cite{shmoys1993approximation} and has later been extended to clustering problems by \cite{bera2019fair,bercea2018cost}. 

     Let us define a flow network $(G,c,a,d)$
     with non-negative capacities $c$, $a$ denotes the cost on each edge, and $d$ denotes the demands on vertices. 
     The directed graph $G$ has a source node $s$, and a sink node $t$ with vertex demands $d_s$ and $d_t$ given by $n$ and $-Y$ respectively. There are mainly three types of vertices in $V - \{s,t\}$ i.e., $V = V_{\cP} \cup V_S  \cup_{h }V_S^h $. We define the vertex sets along with demands $d_v,v\in V$ as following. 
\begin{align*}\small
     V_\cP &= \cup_{h \in \cH} V_\cP^h, V_\cP^h =\{ v_{j,h} : j \in \cP, h\in \cH \} (d_{j,h}:= 0)  \textbf{ Points $\cP$} \\
     V_S^h &=\{ v_{i,h} : i\in S, h\in \cH \} (d_{i,h} := \text{-} \lfloor y(i,h )\rfloor ) \textbf{ Cluster $i$, group $h$} \\ 
    V_S &:= \{v_{i} : i\in S\} (d_i:= - Y(i) ) \textbf{ Cluster $i$ } \\
\end{align*}
Now, we define the edges on the flow network i.e., edges between the vertices $V_\cP, \cup_{h \in \cH}V_S^h$, between vertices $\cup_{h \in \cH}V_S^h$ and $V_S$, and vertices $V_S, t$ along with their non-negative capacities $c$. 

% Note that the cost of edges is given $a_e$ for an edge $e$, and we assume that the edges have zero cost if the cost is not given.   

\textbf{ Points $\cP$ to be assigned}
\begin{equation*}
        E_\cP := \{(s,j ) : j\in V_\cP \} (c_{i,j}:=1)
     % \cup_{h} E^h ,
\end{equation*}
\textbf{ Assignment of $\cP_h$ to cluster $i$} 
\begin{equation*}\small
     E^h := \{ (v_{i,h},v_{j,h}) :  v_{i,h}\in V_S^h,  v_{j,h}\in V_P^h \} (c_{i,j} :=1, a_{i,j} = d(i,j) )
\end{equation*}
\textbf{ Merging of the groups in cluster $i$}
\begin{equation*}\small
    E_S := \{ (v_{i,h},v_i) : v_{i,h} \in V_S^h,  v_{i} \in V_S  \} (c_{i,j} := y(i,h)- \lfloor y(i,h) \rfloor )   
\end{equation*}
\textbf{ Total number of the points clustered}
\begin{equation*}
        E_t := \{ (v_i,t) :   v_{i} \in V_S\} (c_{i,j}:=y(i)- \lfloor y(i) \rfloor ) 
\end{equation*}
We now define $G$ as follows,
\begin{align*}
       V  &:= V_\cP \cup V_S \cup_{h} V_S^h  \cup \{s,t\}, E := E_\cP \cup E_S \cup_{h} E^{h}  \cup E_t 
     % a_e &=  d_{i,j} \forall e= (v_{i,h}, v_{j,h}) \in E^h, 0 \text{ otherwise } 
\end{align*}
Combining Lemma~\ref{lemma:rounding_final}, and \ref{lemma:obj_rounded} we can conclude that, there exists an integral solution $X$ such that the cost of the solution is at most $3$\optf{} for any feasible solution $x$ to the LP~(\ref{lp:rfa}-\ref{eq:endrfa}) since $x_{i,j} = 0 $ for any $d(i,j)>3$\optf{}.   
% Therefore, there exists a rounded solution $X$ to our feasible LP solution $x^*$ with a cost of at most $3$\optf{} 
\end{proof}

\begin{proof}[Proof of Lemma~\ref{lemma:obj_rounded}]
    Since the \textsc{MaxFlow} network $F(x)$ for any given $x$ and instance $\cI$ has integral capacities, and demands, we can say that there exists an integral flow $f$.
    Therefore, we can construct the rounded solution $X$ to the clustering instance as follows : for each $i \in S, j \in \cP_h$,
    $$X_{i,j} = f_e ,  e = (v_j ,v_{i, h}), \text{ where } v_j \in V_\cP^h, v_{i,h} \in V_S^h .$$
    Since the flow $f$ is integral, this gives us an integral assignment of all points $j \in \cP$ to centers $S$. 

    The last inequality is due to the fact that cost of the \textsc{MaxFlow} integral flow is at most any feasible flow in the network. Moreover, each vertex $v \in V_S$ has a demand of $\lfloor y(i) \rfloor$ i.e., at least $\lfloor y(i) \rfloor$ number of points that are assigned to it, and the outgoing flow of $v$ is at most $1$, therefore, we can say that
    $$  \lfloor y(i) \rfloor + 1 \geq  |C_i|  \geq \lfloor y(i) \rfloor, \quad \quad \forall i \in S. $$
    Similarly, each vertex $ v \in V_S^h$ has a demand of $ \lfloor y(i,h) \rfloor $, and an outgoing flow of at most $1$ unit, therefore, we can say that center $i$ gets at least $\lfloor y(i,h) \rfloor$ points of color $h$, 
    $$ \lfloor y(i,h) \rfloor + 1 \geq |C_i| \geq \lfloor y(i,h) \rfloor, i \in S, h\in \cH.  $$
Therefore, based on the rounding algorithm \textsc{MinCostNetworkRound}, we can say that the following holds,
% Therefore, we can say that the following is true since the rounding of \cite{bercea2018cost} satisfies \eqref{ineq:rounding_color}. 
% \begin{equation} \label{ineq:cih}
%   l_h  \lfloor \sum_{j \in \cP} x_{i,j}^* \rfloor  \leq       \sum_{ j \in \cP_h}X_{i,j}  \leq u_h \lceil \sum_{j \in \cP} x_{i,j}^*  \rceil
% \end{equation}
\begin{equation} \label{ineq:ci}
    \sum_{j \in \cP} x_{i,j}^*   -1  \leq |C_i| = \sum_{j \in \cP}X_{i,j}  \leq  \sum_{j \in \cP} x_{i,j}^*  +1, \forall i\in S
\end{equation}
\begin{equation} \label{ineq:cih}
     \sum_{j \in \cPh} x_{i,j}^*  -1  \leq |C_{i,h}(\chi)| = \sum_{j \in \cPh}X_{i,j}  \leq \sum_{j \in \cP} x_{i,j}^*  +1, \forall i,h 
\end{equation}
\end{proof}

\begin{lemma} \label{lemma:rounding_final}
    For every feasible solution $x$ to satisfying \cref{lp:rfa}-\cref{eq:endrfa}, there exists a valid flow circulation in the corresponding \textsc{MaxFlow}. 
\end{lemma}

\begin{proof}
    Let the corresponding \textsc{MaxFlow} flow network corresponding to a feasible solution $x$ be $F(x)$ where $F(x)$ is constructed as shown in Figure~\ref{fig:enter-label}. Notice that $x$ induces a feasible flow to $F(x)$, where flow on each edge is defined as follows, 
    \begin{enumerate}[noitemsep,nolistsep] 
        \item The flow on each of the edges $e \in E_\cP$ is given by $f_e =1$, and for each of the edges $e = (v_{j} , v_{i,h}) \in E^h$ is given by $f_e = x_{i,j}$. Therefore, flow is conserved at vertex $s$, and for each vertex $j \in V_{\cP}^h$ and group $h \in \cH$, \begin{equation*}
            f_{\text{in}}(j) = 1 =  \sum_{ i \in V_S^h}x_{i,j} =  f_{\text{out}}(j)  =\sum_{i \in S} x_{i,j}=1 .
        \end{equation*}
        \item The flow between the edges of $V_S^h$ and $V_S$ is given by $f_e = y(i,h) - \lfloor y(i,h) \rfloor $ for each $e = (v_{i,h},v_i)$, $v_{i,h} \in V_S^h, v_i \in V_S$. Hence, we can say that for each vertex $v \in V_S^h$ the flow is conserved i.e.,
       \begin{equation*}
           f_{\text{in}}(v) + d_v = \sum_{j : j\in \cP_h }x_{i,j} + d_v = y(i,h) - \lfloor y(i,h) \rfloor = f_{\text{out}}(v). 
       \end{equation*}
        \item The flow between the edges of $V_S$ and $t$ is given by $f_e = y(i) - \lfloor y(i) \rfloor $. Flow conservation at vertices $v \in V_S$ is given by,
        \begin{align*}
            f_{\text{in}}(v) &= \sum_{ h \in \cH } y(i,h) - \sum_{ h \in \cH} \lfloor y(i,h)\rfloor + d_v \\
            &= y(i) - \sum_{ h \in \cH}  \lfloor y(i,h) \rfloor  - Y(i) \\
            &= y(i) - \lfloor y(i) \rfloor  = f_{\text{out}}(v)
        \end{align*}
    \end{enumerate}
\end{proof}

\section{More Discussion About the Noise Model and Its Relation to Previous Noise Models}
%%%%%%%%%%%%%%%%%%%%%%%%%%%%%%%%%%%%%%%%%%%%%%%%%%%%%%%%%%
%%%%%%%%%%%%%%%% PFC COMPARISON %%%%%%%%%%%%%%%%%%%%%%%%%%
%%%%%%%%%%%%%%%%%%%%%%%%%%%%%%%%%%%%%%%%%%%%%%%%%%%%%%%%%%
\subsection{Drawbacks of the Noise Model of Probabilistic Fair Clustering \cite{esmaeili2020probabilistic}}\label{app:pfc_discussion}
We provide an example to show the drawbacks of the probabilistic model of group uncertainty introduced in \citet{esmaeili2020probabilistic}. Their theoretical guarantees for robust fair clustering only guarantee to satisfy the fairness constraints in expectation. However, the realizations can be arbitrarily unfair. 
We illustrate this using an example.
Consider a set of $14$ points as shown in the \cref{fig:negative_example} where each point is assigned to either the red or blue group, each with a probability of $1/2$. Any clustering of these points is fair in expectation. However individual realizations can be unfair. Specifically, since the joint probability distribution is not known (in fact, it is not incorporated at all in the probabilistic model of \citet{esmaeili2020probabilistic}) the realizations could be as shown in the figure where all points in a cluster take on the same color simultaneously in a realization. This shows that the probabilistic model may return clusters that can be fair (proportional) in expectation but completely unfair (unproportional) in realization.    

% Therefore, we show that the probabilistic model 
% may not be practical. 

\begin{figure}[H]
    \centering
    \includegraphics[width=1.1\textwidth]{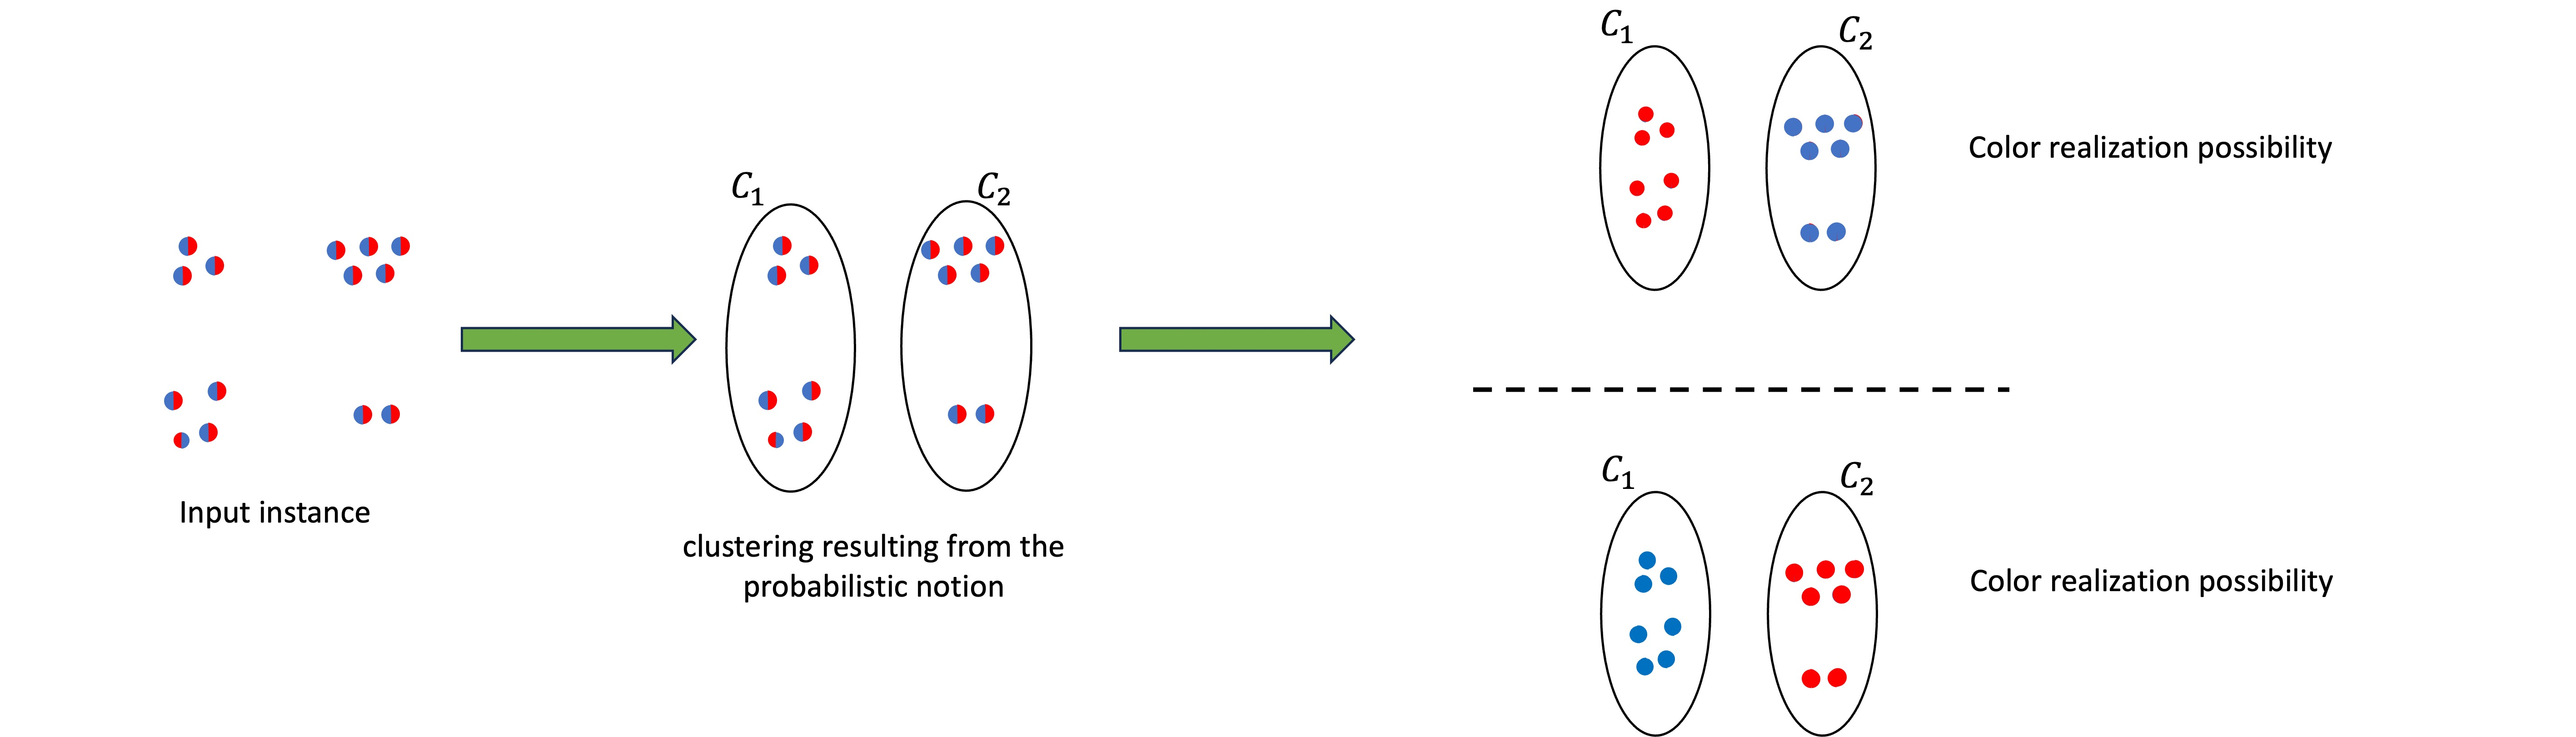}
    \caption{An instance of \fc{} with $14$ points where each point has the probabilities $p_{j}^{\text{red}}=p_{j}^{\text{blue}}=\frac{1}{2}$. Here $p_{j}^{\text{red}}$ and $p_{j}^{\text{blue}} \forall j \in \cP$ denote the probability that point $j$ belong to red and blue groups respectively. Note how the probabilistic fair clustering satisfies fairness in expectation. However, the two realizations shown demonstrate that color proportionality can be completely violated. }
    \label{fig:negative_example}
\end{figure}

%%%%%%%%%%%%%%%%%%%%%%%%%%%%%%%%%%%%%%%%%%%%%%%%%%%%%%%%%%
%%%%%%%%%%%%%%%% CHABRA COMPARISON %%%%%%%%%%%%%%%%%%%%%%%
%%%%%%%%%%%%%%%%%%%%%%%%%%%%%%%%%%%%%%%%%%%%%%%%%%%%%%%%%%
\subsection{More Discussion About the Noise Model of \cite{Chhabra23:Robust}}\label{app:chhabra_discussion}
% \SD{Edit this.}
We provide an example to show the drawbacks of the noise model of group uncertainty introduced by \citet{Chhabra23:Robust}. Their noise model assumes that only a subset of the points are affected by the adversary but they do not specify how can one access this subset. In their experiments, they generate this subset using random sampling. Specifically, they independently sample each point with probability $0.15$ to obtain a subset of points $\cP' \subseteq \cP.$ However, we can easily construct examples where their random sampling method with probability $\approx 0.99$ can never return some subsets. We illustrate this using an example. Consider an instance of \fc{} as shown in \cref{fig:negative_example_two} where only a subset of points have incorrect memberships according to \citet{Chhabra23:Robust}. Their sampling process selects a subset (comprising 10\% of the points) by randomly sampling each point independently with a probability of $0.1$. As a result, out of $160$ points $16$ points are perturbed in expectation. However, this does not capture scenarios where all perturbations occur within a subset of points (as shown in the left side of \cref{fig:negative_example_two}) as the probability of such an event is close to $0$, precisely $0.0002$. On the other hand, our model considers for all possible subsets with $16$ points.  As a result, we can model the scenarios where all the incorrect memberships occur in a single group or more generally all possible combinations across the two groups. 

% Note that this results in the scenario where $4$ points are sampled from each of the two groups with a probability $\approx 0.99$. 
\begin{figure}[H]
    \centering
    \includegraphics[scale=0.4]{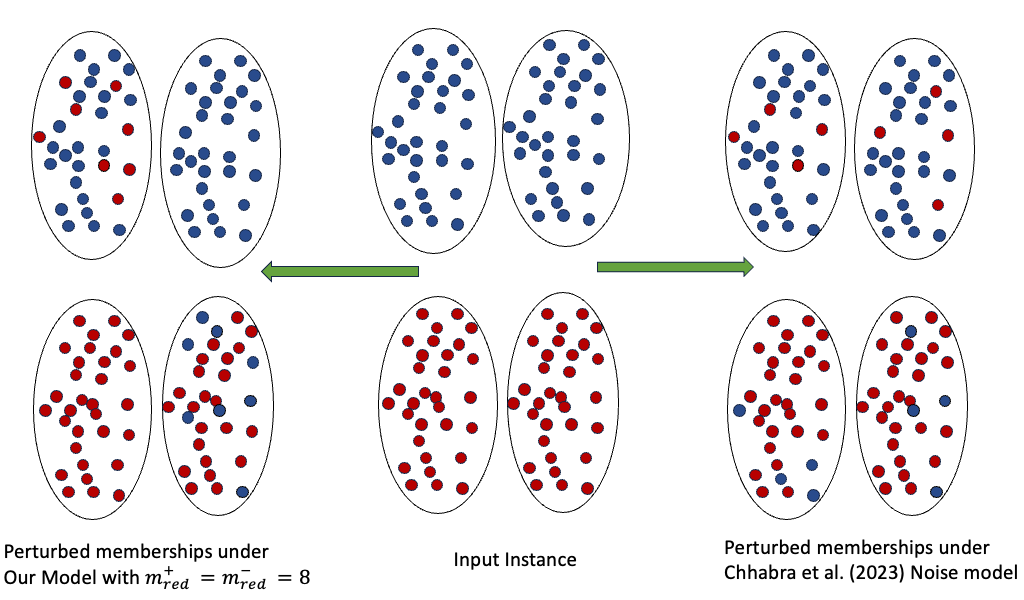}
    \caption{Consider an instance of \fc{} with $n=160$ points, where $10\%$ of the points have incorrect memberships. \citet{Chhabra23:Robust} perturbs a subset (comprising 10\% of the points) by randomly sampling each point independently with a probability of $0.1$. As a result $16$ points are perturbed in expectation. However, this does not capture scenarios where all perturbations occur within a subset of points as shown on the left side. This is because the probability of such an event is $\approx 0$. On the other hand, our model considers for all possible subsets with $16$ points, thereby covering all possible scenarios.}
    \label{fig:negative_example_two}
\end{figure}

\section{Additional Details on our Experimental Setup \& Experimental Results}\label{app:experiments}

We describe additional details about libraries and hardware used in Section~\ref{app:experiments-setup}, and provide additional experimental runs varying parameters in Section~\ref{app:experiments-results}.

%\sd{give the definition of the evaluation metrics which is the fairness violation and the clustering cost under $k$-center objective}

\paragraph{Evaluation Metrics}
\SD{This para must be changed since it has $T$ and the model has changed since!!}
Fairness violations are computed in one of two ways.
For robust and deterministic we report the fairness violation as in \eqref{eq:robust_fair} in excess of $T$.
For probabilistic clustering, the error model of is different. Here, each point's color is correct with some probability $p_{acc}$, which we fix to $1-m$ thus corrupting the same fraction of points $m$, in expectation. We will illustrate that simply taking the marginals $p_{acc}$ into account is far from sufficient to guarantee a fair clustering after label realizations. This is because there may be significant correlations in the points' label corruptions resulting in large shifts in the color representation in any given cluster. To this end we consider the following simple scenario which respects the marginals and induces positive correlation in different points' label errors: for each pair of color and cluster, sample $X \sim Ber(p_{acc})$ and simultaneously flip all color labels if and only if $X=1$ to an alternate color $c'$ sampled uniformly at random. If $X=0$, then do nothing.

\subsection{Experimental Setup}\label{app:experiments-setup}
The experiments are run on Python 3.6.15 on a commodity laptop with a Ryzen 7 5800U and 16GB of RAM. The linear program (LP) in the algorithms are solved using CPLEX 12.8.0.0 and flow problems are solved using \texttt{NetworkX} \cite{hagberg2013networkx} 2.5.1. In total, we solve $3 \times 20 + 3 \times 2 = 66$ fair clustering instances (60 robust clustering instances, 3 probabilistic, and 3 deterministic) in 78 minutes.
The associated LPs are solved using \texttt{CPLEX} \cite{nickel2022ibm} 12.8.0.0. Our code implementation builds on the code of \cite{dickerson2023doubly}.

\subsection{Additional Experimental Results}\label{app:experiments-results}
Like before, the baselines' lines intersect because $p_{acc} \approx 1$ suggests that similar clustering assignments can solve both instances. We do not check the probabilistic baseline on \cens, which has 3 colors, because the main result of \cite{esmaeili2020probabilistic} applies to the 2-color setting. 
We further make a note that for all the plots, the fairness violations plotted never exceed $2/m_{out}$, which is our theoretical guarantee. For example, when $m=0.005$ then $2 / m_{out} = 2 / (0.005 \cdot 6000) = .06$ for BAE and BAPE. 
\begin{figure}
    \centering
    \includegraphics[width=\textwidth]{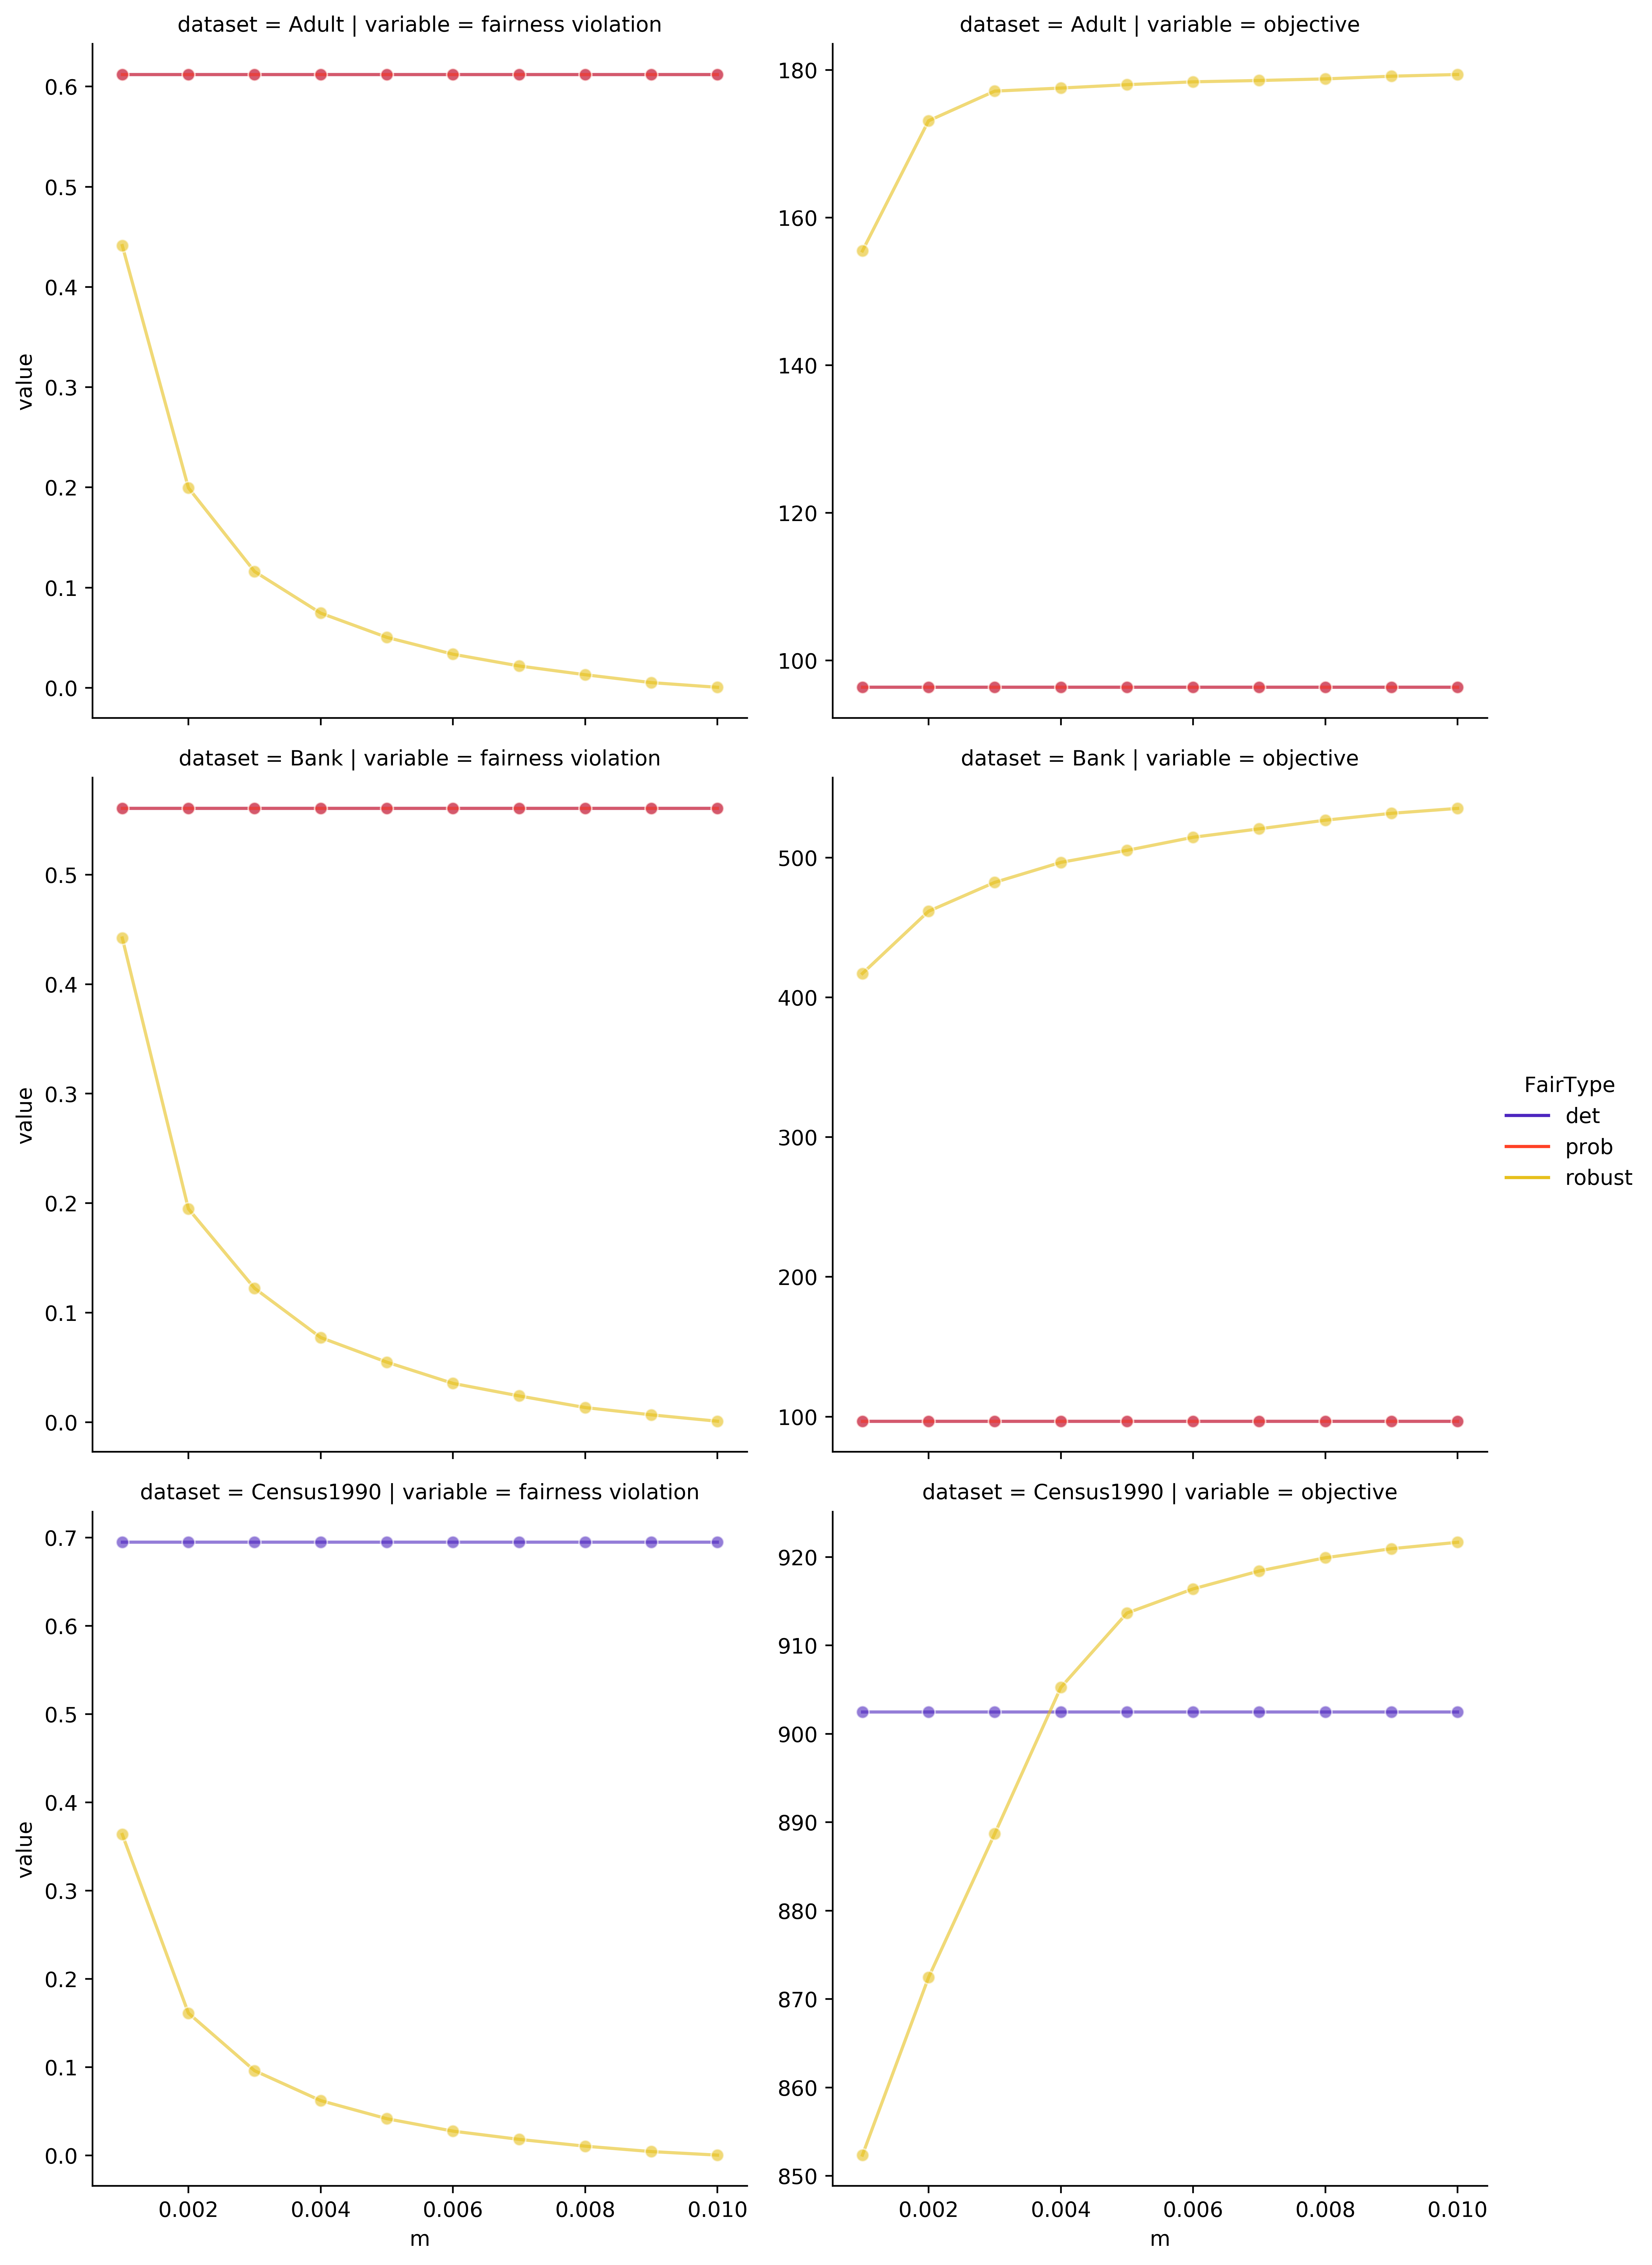}
    \caption{Experiments varying $m$ on all three datasets. Note it is possible for the robust algorithm to outperform the baselines' objective due to the presence of $T$ which loosens the fairness constraints.}
    \label{fig:enter-label}
\end{figure}

\begin{figure}
    \centering
    \includegraphics[width=\textwidth]{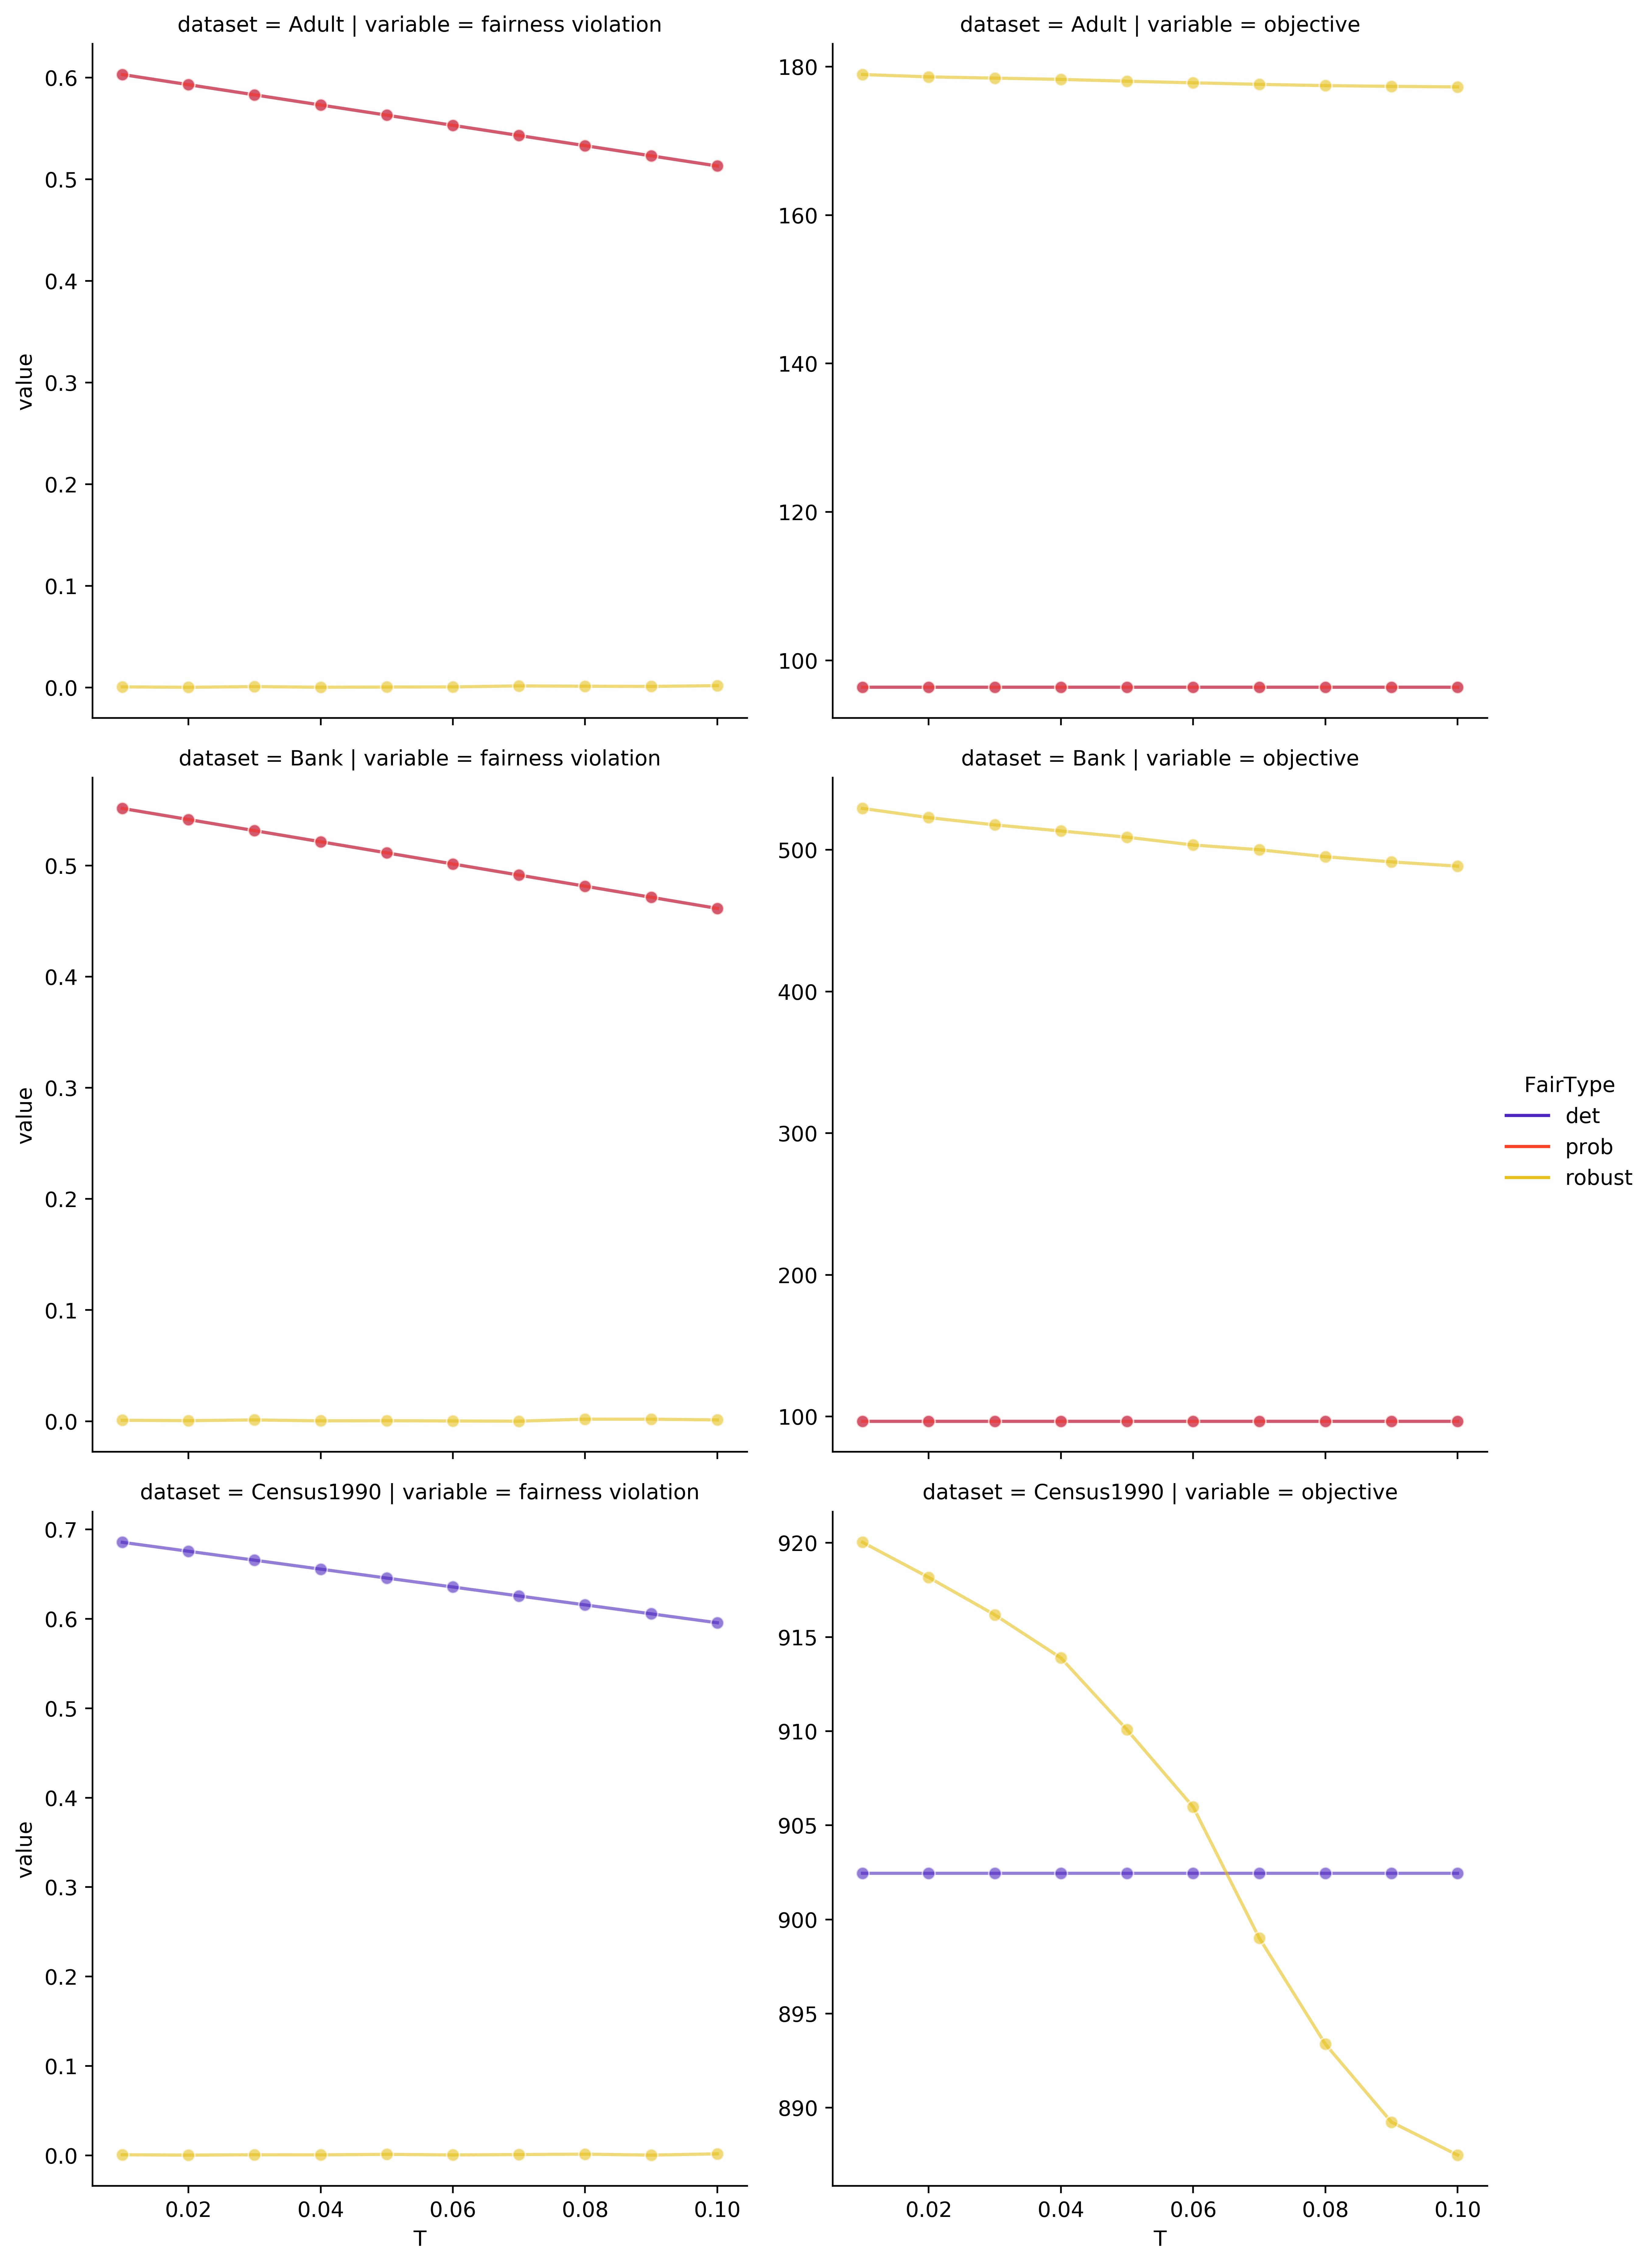}
    \caption{Experiments varying $T$ on all three datasets.
    Note it is possible for the robust algorithm to outperform the baselines' objective due to the presence of $T$ which loosens the fairness constraints.
    }
    \label{fig:enter-label}
\end{figure}
  % \end{minipage}
